# Supplementary material for: HyDA-Vista: Towards Optimal Guided Selection of k-mer Size for Sequence Assembly
Source: arXiv:1408.5592 source file (2014-08-24)
Supplement: Supplementary file 1 [file supplement.tex]

z\section*{Appendix}  \label{sec:supplement}

We now give the definition and construction for the ordered binary tree used in the maximal sequence landscape construction algorithm.  Given an integer array $\L$, we build an  ordered binary search tree for all consecutive pairs of integers in the list.   We create a leaf node for each pair of integers, and create a set of parent nodes at each level of the tree. Each parent node contains the interval $[min, max]$ that corresponds to the largest integral range containing the labels of the child nodes.  See Figure \ref{fig:tree} for an illustration of this.  This is a complete binary tree with $n - 1$ leaves so  the total number of nodes is $2(n - 1) - 1$. Hence, the construction of the tree takes $O(n)$-time and $O(n)$-space.  Lastly, we note that the height of the tree is $O(\log n)$. 

\begin{figure}
\caption{An ordered binary tree of all the consecutive intervals the array $\L = [3,6,1,3,5,5,8,7,1]$. This data structure is used to efficiently solve the  \textsc{Largest Interval Problem}.  See the proof of Theorem \ref{lip}.}
\label{fig:tree}
\begin{center}
\includegraphics[scale=.7]{figures/tree}
\end{center}
\end{figure}

Next, we show that solving the  \textsc{Largest Interval Problem} for a given list $\L$ can be done in $O(\log n)$-time and $O(n)$-space using an ordered binary search tree of all the consecutive intervals in $L$.  

\begin{definition} Given an array of integers $\L$ of size $n$, index $i \in [1,n]$, and threshold $\alpha$, the \textsc{Largest Interval Problem} aims to find the largest interval $[a,b] \subseteq [1,n]$ such that $i \in [a,b]$ and $\L[k] \geq \alpha$ for all $k \in [a,b]$. \end{definition}

We now prove the following theorem.  

\begin{theorem} \label{lip} Given an ordered binary tree of all the consecutive intervals in $\L$, the \textsc{Largest Interval Problem} can be solved in $O(\log n)$-time and $O(n)$-space.  \end{theorem}

\begin{proof}  For a given index $i$ and threshold $\alpha$, we use the ordered binary search tree to find the largest interval $[a, b]$ around $i$, where $\L[j] \geq \alpha$ for all $j \in [a, b]$.    First, we assume that there exists two leaves containing $\L[i]$.  Let $\ell_{i1}$ and $\ell_{i2}$ be the leaves that have the minimum and the maximum integer, respectively.   In order to find $a$, we traverse the tree from $\ell_{i1}$ to the root until we reach the root or a node that has a label with property $\alpha \not\in [min, max]$, and then traverse down tree taking lefthand edges to a leaf node is reached. The minimum of this leaf node is $a$.  Next, we can find the value of $b$ using the same approach, with the exception that we start the traversal from $\ell_{i2}$, and traverse up the tree while $alpha \not\in [min, max]$.  Then we traverse down the tree taking the righthand edges until a leaf node is reached.  The maximum of at this leaf node is $b$.  

When there exists only a single leaf node containing $\L[i]$ then we are the beginning or the end of the list and only $a$ or $b$ needs to be found. Therefore, at most four traversals from a leaf to the root of the tree are needed, and since the height of tree is $O(\log n)$, the total running time of the algorithm is $O(\log n)$-time. \hfill \qed \end{proof} 

Corollary \ref{lemma2} follows directly from Theorem \ref{lip}. 

The results in the main body of the paper were focused on the construction of the maximal sequence landscape from the {\em self} sequence landscape.  Here, we will prove a stronger result that states the maximal sequence landscape for the sequence landscape constructed for $s$ and $t$ can be constructed in $O(n + m \log n)$-time and $O(m)$-space, where $n$ is the length of $s$ and $m$ is the length of $t$.   First, we prove an intermediate result concerning the \emph{silhouette} of a sequence landscape, which is the maximal sequence landscape without any constraint on frequency of each mountain.  We remind the reader that each mountain in the maximal sequence landscape has frequency greater than one which is not the case for the silhouette. % Finally, the \emph{ height of the maximal landscape} at a specific index i $h(L^*_{t|s},i)$ is the height of the highest mountain that covers $i$ or: $h(L^*_{t|s},i) = h(S_{L_{t|s}}(i))$.

\begin{lemma} \label{lem:general} The silhouette of the sequence landscape $\L_{t|s}$ of string $t$ with respect to string $s$ can be built in $O(n + m \log n)$-time and $O(n)$-space, where $n$ is the length of $s$ and $m$ is the length of $t$. \end{lemma}

\begin{proof} We present a constructive proof. Given $s$, we construct $\SA_s$ and $\LCP_s$.  This construction can be done in $O(n)$-time and $O(n)$-space \cite{ks2006}. Next, we define another auxiliary array of $s$, denoted as $\SP_s$, that is used to efficiently traverse $\SA_s$ in a specific order. $\SP_s[i]$ contains the index of the suffix in $\SA_s$ that is obtained by removing first letter from $\SA_s[i]$. We note that $\SP_s$ can be computed in $O(n)$-time and $O(n)$-space by scanning the $\SA_s$ once. Table \ref{fig:sp} illustrates this construction of $\SP_s$. $\SP_s$ can be interpreted as an array that saves a pointer to the next entry in Burrow's Wheeler transform of $s$.

Given these arrays, we process $t$ from one letter at a time. We let $b_i$ and $e_i$ be indices of the string $t$, i.e., $b_i \leq t_i$, and $b_i \in [1, n]$ and $e_i \in [1, n]$. Lastly, we denote $t[b_i,e_i]$ as the current substring of $t$ that we are processing at the $i$'th iteration of the algorithm.  We note that $b_0$ and $e_0$ are initialized to zero at the beginning of the algorithm. At iteration $i$ of algorithm,  we are trying to match the largest substring of $t$ containing the $i$'th character with a substring in $s$. In order to accomplish this, we need to search for the substring $t[b_i,e_i] = t[b_{i-1},e_{i-1}] t_i$ in  $\SA_s$. Since we have already matched first $e_{i-1}-b_{i-1}$ characters of $t[b_i,e_i]$ with some entry in $\SA_s(t[b_{i-1},e_{i-1}])$ (possibly none), and the starting and ending index for binary search in $\SA_s$ is already saved, this can be done in $O(\log n)$. To see this we must consider two cases that arise when processing $t[b_i,e_i]$ at iteration $i$.
\begin{enumerate}
\item[(a)] If $t[b_i,e_i]$ is contained in $\SA_s$ then the silhouette is updated, $e_i$ is incremented, and the starting and ending indices of the search interval for $\SA_s$ are updated for next iteration.  The search interval can be updated using binary search on $\SA_s$.
\item[(b)] If $t[b_i,e_i]$ is {\em not} contained in $\SA_s$, then one letter at a time is eliminated from the beginning of $t[b_{i-1},e_{i-1}]e_{i}$ until it is found in $\SA_s$, or the null string is reached.  We let $p'$ denote the string obtained from eliminating the first character from the current string.  The search interval is no longer valid for $p'$ since we removed the first character, and therefore, we need to efficiently find the search interval for $\SA_s$.  To find the correct search interval, we locate the index of the suffix in $\SA_s$ that has $p'$ as a prefix,  we denote this index as $sp$, and find the interval around $sp$ where each suffix in this interval has $p'$ as a prefix.  This is the new search interval.  The index $sp$ can be found in constant time using $\SP_s$ since $sp = \SP_s[\SA_s [t[b_{i-1},e_{i-1}]]]$, and it follows from Theorem \ref{lip} that the interval can be found in $O(\log n)$-time. 
\end{enumerate} 

In (a) the silhouette is ascending and in (b) the silhouette is descending.  Since each time the silhouette ascends we process a letter from $t$, and the number of times the silhouette descends is equal to the number of times it ascends, the number of ascents or descents is $O(m)$.  Since each ascent or descent requires $O(\log n)$-time the algorithm requires at most $O(m \log n)$-time after the construction of the data structures.   All data structures require $O(n)$-time for construction, and $O(n)$-space.  Thus, the algorithm requires $O(n + m \log n)$-time and $O(n)$-space.  \hfill \qed  \end{proof}

\begin{theorem} \label{thm:general} The maximal sequence landscape of string $t$ of size $m$ with respect to string $s$ of size $n$ can be built in $O(n + m \log n)$-time and $O(n)$-space. \end{theorem}

\begin{proof} The construction of the maximal sequence landscape is identical to the construction of the silhouette with the addition that the frequency of each mountain has to be checked in order to determine if it is greater than one.   Determining whether the frequency is greater than one can be accomplished in constant time using the $\LCP_s$, i.e., if $\LCP_s[\SA_s[t[b_i,e_i]]+1]$ or $\LCP_s[\SA_s[t[b_i,e_i]]-1]$ is greater than or equal to $e_i - b_i$ then we can conclude $t[b_i,e_i]$ has frequency greater than one at iteration $i$ of the algorithm.  Hence, this construction takes $O(m + \log n)$-time and $O(n)$-space by Lemma \ref{lem:general}.  \hfill \qed \end{proof}

%$5n \times \log n +O(c)$ bits 
